# Supplementary material for: Mammalian cochlea as a physics guided evolution-optimized hearing sensor
Source: arXiv:1409.0655 source file (2014-11-18)
Supplement: Supplementary file 1 [file LorimerGomezStoopAppendix.pdf]

# Appendix for
# Mammalian cochlea as a physics guided evolution-optimized hearing sensor

Tom Lorimer, Florian Gomez, Ruedi Stoop
Institute of Neuroinformatics, University of Zurich and ETH Zurich,
Winterthurerstrasse 190, 8057 Zurich, Switzerland

## Periodic signals from natural dynamics

It seems justified to ask where the origin of this *abundance* of periodic signals generated in the animal world may be? Here we put forward that observed periodicity may often emerge even from a less specialized source: from an underlying chaotic process. In the animal world, the dynamical processes are generally much more complicated and usually nonlinear. A classical example are pattern generators taken in a very general sense. If we take the animal gaits as the illustrative example, we may ignore in this context that their generating frequencies are somewhat low, seen from an auditory angle. As a tendency young animals make strange - as we will interpret it: chaotic - movements. Chaos provides the basic basin from which partial motions are selected, offering a great richness of choices to the system [1, 2]. Influence of living conditions or conditions arising from the survival paradigm then constrains the selection in an easy to grasp manner to simpler, less costly behavior, by acting as limiting conditions that change chaotic into periodic behaviors, a paradigm known under the name of limiter control [3, 4, 5, 6]. It can moreover be inferred that the energy spent in a limiter-controlled periodic state is minimal [7]. For animals, load, weight or speed may act as such limiters; seen for instance in the transition from walk (period 4) to trot (period 2) 'gaits' in quadrupeds under the constraint of increasing speed. As a result, periodic signals are not restricted to simple physical oscillators, they are also the most basic sound signatures of more complex systems from the animal world. In Fig.1 we illustrate this by taking, similarly to Ref. [3], two joints that would move chaotically, if not limited by elastic forces active as soon as one has crossed a certain threshold. Without loss of generality, we may restrict the control to the upper joint, where we introduce a spring-type energy $V = \frac{1}{2}k[\theta_1 - \mathrm{sign}(\theta_1)\theta_0]^2$ that only becomes active for $|\theta_1| > |\theta_0|$. The addition to Hamilton's equations $\propto k\,[\theta_1 - \mathrm{sign}(\theta_1)\theta_0]$, for $|\theta_1| > |\theta_0|$ offers, by a choice of $\theta_0$ to force the system onto a desired periodic orbit.

When animals extract information from a complex environment, most of the time they will be interested in data too regular to be of accidental nature. This is because such signals are likely to be generated by conspecifics, by potential predators or by preys.

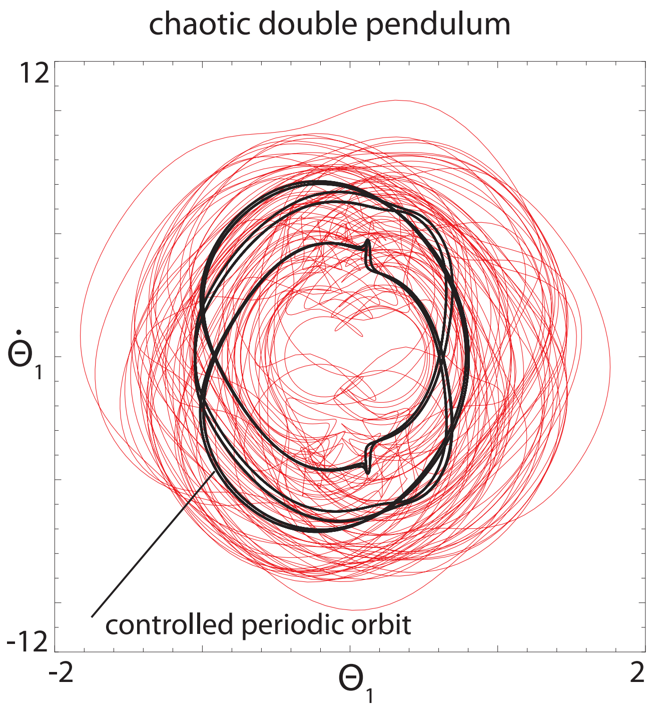


Figure 1: Complex biological system with a limiting conditions forcing chaotic motion into periodic behavior. Free (red) vs. limiter-controlled (black) orbits of a double pendulum model of a double-joint limb. A limiter implemented by a spring becomes active whenever an angle exceeds a threshold in one of the joints.

## References

Shinbrot, T., Grebogi, C., Ott, E., Yorke, J.A. Using small perturbations to control chaos. *Nature* **363**, 411-417 (1993).

Boccaletti, S, Grebogi, C., Lai, Y.C., Mancini, H., Maza, D. The control of chaos: theory and applications. *Physics reports* **329**, 103-197 (2000).

Corron, N.J., Pethel, S.D., Hopper, B.A. Controlling chaos with simple limiters. *Phys. Rev. Lett.* **84**, 3835-3838 (2000).

Corron, N.J., Hopper, B.A., Pethel, S.D. Limiter control of a chaotic RF transistor oscillator. *Int. J. Bifurcat. Chaos* **13** 957-961 (2003).

Wagner, C., Stoop, R. Renormalization approach to optimal limiter control in 1-d chaotic systems. *J. Stat. Phys.* **106**, 97-107 (2002).

Stoop, R., Wagner, C. Scaling properties of simple limiter control. *Phys. Rev. Lett.* **90**, 154101 (2003).

Christen, M., Ott, T., Kern, A., Stoop, N., Stoop, R. Periodic economic cycles: The effect of evolution and control. *J. Stat. Mech.: theory and experiment* **11**, P11013 (2005).
